# Supplementary material for: Learnable Strategies for Bilateral Agent Negotiation over Multiple Issues
Source: arXiv:2009.08302 source file (2022-01-07)
Supplement: Supplementary file 1 [file OldAppendix.tex]

\begin{table*}
    \centering
    \resizebox{.98\textwidth}{!}{
    \begin{tabular}{p{0.07\textwidth} p{0.1\textwidth}p{0.1\textwidth}
    p{0.1\textwidth}p{0.1\textwidth}
    p{0.1\textwidth}p{0.1\textwidth}
    p{0.1\textwidth}p{0.1\textwidth}}
    \hline
    Metric & \multicolumn{2}{c}{ANESIA} & \multicolumn{2}{c}{AgentGG} & \multicolumn{2}{c}{KakeSoba} & 
    \multicolumn{2}{c}{SAGA}  \\
    \hline
    & $|B| = 5$ & $|B| = 10$   
    & $|B| = 5$ & $|B| = 10$  
    & $|B| = 5$ & $|B| = 10$
    & $|B| = 5$ & $|B| = 10$ \\
    \hline
    \multicolumn{9}{c}{\textbf{Holiday Domain}} \\
    \hline
    $T_{\it avg}$  &  39.75 $\pm$ 26.19 & 35.6 $\pm$ 28.19 & 36.52  $\pm$ 48.97 & 26.27  $\pm$ 29.49 & 32.93 $\pm$ 49.04 & 19.98 $\pm$ 28.8 &  11.72 $\pm$ 18.98 & 15.08 $\pm$ 23.13 \\
    
    $R_{\it avg}$  &  476.81 $\pm$ 847.48 & 259.35 $\pm$ 453.3 &  1224.04  $\pm$ 1770.48 & 532.77  $\pm$ 841.16 & 1066.18 $\pm$ 1710.8	 & 414.51 $\pm$ 719.58 & 32.3 $\pm$ 83.79 & 238.18 $\pm$ 783.88\\
     
     $P_{\it avg}$  &  \textbf{0.15 $\pm$ 0.57} & \textbf{0.17 $\pm$ 0.26} & 0.4  $\pm$ 0.46 & 0.35  $\pm$ 0.44 & 0.28 $\pm$ 0.44 & 0.17 $\pm$ 0.34 & 0.23 $\pm$ 0.37 & 0.31 $\pm$ 0.42 \\
     
      $U_{\it soc}$  & \textbf{1.79 $\pm$ 0.81} & \textbf{1.72 $\pm$ 0.78} & 1.25  $\pm$0.66 & 1.33  $\pm$ 0.62 & 1.41 $\pm$ 0.63 & 1.57 $\pm$ 0.49 & 1.49 $\pm$ 0.53 & 1.39 $\pm$ 0.59\\
    
    $U_{\it ind}$  & 0.46 $\pm$ 0.42 & 0.51 $\pm$ 0.39 & 0.67  $\pm$0.37 & 0.73  $\pm$0.34 & 0.73 $\pm$ 0.34 & 0.8 $\pm$ 0.26	& 0.65 $\pm$ 0.24 & 0.61 $\pm$ 0.29\\
    
    $U_{\it ind}^s$  & \textbf{0.88 $\pm$ 0.11} & \textbf{0.88 $\pm$ 0.01} & 0.86  $\pm$0.13 & 0.88  $\pm$0.07 & 0.87 $\pm$ 0.13 & 0.87 $\pm$ 0.11 & 0.73 $\pm$ 0.1	 & 0.71 $\pm$ 0.17\\
    
    $P_{succ}$ & 0.56 & 0.64 & 0.79 & 0.83 & 0.84 &\textbf{ 0.92} & 0.89 & 0.86\\
    \hline
    
    \multicolumn{9}{c}{\textbf{Laptop Domain}} \\
    
    \hline
    
    $T_{\it avg}$ & 36.81 $\pm$28.74 & 37.07 $\pm$ 28.07 & 34.56  $\pm$ 29.14 & 31.13  $\pm$ 28.96   & 24.0  $\pm$ 28.28 & 20.53  $\pm$ 26.94 & 14.2 $\pm$ 23.08  & 12.03 $\pm$ 20.82\\
    
    $R_{\it avg}$  &  256.27 $\pm$ 393.1 & 254.62 $\pm$446.96 & 2840.6  $\pm$ 5055.29 & 2186.61  $\pm$ 4523.85 & 	2292.48  $\pm$ 4559.91 & 2054.73  $\pm$ 4445.48 & 875.89 $\pm$ 3305.07 & 232.84 $\pm$ 1316.79	 \\
    
    $P_{\it avg}$  & \textbf{0.02 $\pm$0.26} & \textbf{0.05 $\pm$ 0.26} & 0.14  $\pm$0.23 & 0.13  $\pm$ 0.22 & 0.07  $\pm$ 0.18	 & 0.07  $\pm$ 0.18	& 0.06 $\pm$ 0.16 & 0.06 $\pm$ 0.17		\\
    
    $U_{\it soc}$  &  \textbf{1.57 $\pm$0.81} &\textbf{ 1.50 $\pm$ 0.8 }& 0.99  $\pm$ 0.71 & 1.07  $\pm$ 0.7 & 1.26  $\pm$ 0.63 & 1.34  $\pm$ 0.62 & 1.45 $\pm$ 0.56	 & 1.48 $\pm$ 0.56 \\
   
    $U_{\it ind}$  & 0.47 $\pm$ 0.48 & 0.5 $\pm$ 0.48 & 0.68  $\pm$0.42 & 0.72  $\pm$ 0.41 & 0.78  $\pm$ 0.33 & 0.77  $\pm$ 0.32 & 0.71 $\pm$ 0.26	 &0.73 $\pm$ 0.28	 \\
    
    $U_{\it ind}^s$  &\textbf{ 0.96 $\pm$ 0.08} & \textbf{0.95 $\pm$ 0.09} & 0.93  $\pm$ 0.1 &  0.94  $\pm$ 0.09 & 0.91  $\pm$ 0.11	 & 0.89  $\pm$ 0.1 & 0.8 $\pm$ 0.07 & 0.82 $\pm$ 0.09	\\
    
    $P_{succ}$ & 0.48 & 0.52 & 0.73 & 0.76 & 0.86 & 0.87 & 0.89 & \textbf{0.89}\\
    
    \hline
    
    \multicolumn{9}{c}{\textbf{Party Domain}} \\
    
    \hline
    
    $T_{\it avg}$  & 47.24 $\pm$ 25.46 & 54.67 $\pm$ 40.18 & 38.85$\pm$ 33.71  & 44.35$\pm$ 27.26 & 41.19 $\pm$ 32.82 & 45.15 $\pm$ 26.6 7 	& 16.11 $\pm$ 23.87 & 23.58 $\pm$ 44.59\\
    
    $R_{\it avg}$  &  213.2 $\pm$ 274.16 & 229.98 $\pm$ 288.62 & 508.04$\pm$ 607.31 & 673.01$\pm$ 682.91	& 473.42 $\pm$ 560.71	& 627.69 $\pm$ 652.17 & 135.17 $\pm$ 347.58	 & 209.67 $\pm$ 514.01		\\
    
    $P_{\it avg}$  & \textbf{0.15 $\pm$0.42} & \textbf{0.18 $\pm$0.4} & 0.39$\pm$ 0.43	&  0.37$\pm$ 0.46	& 0.4 $\pm$ 0.46	 & 0.36 $\pm$ 0.46 & 0.21 $\pm$ 0.35 & 0.22 $\pm$ 0.39 \\
    
    $U_{\it soc}$  & \textbf{1.41 $\pm$ 0.6 }& \textbf{1.34  $\pm$ 0.59 }& 0.97$\pm$ 0.64	 & 1.0$\pm$ 0.69 & 0.96 $\pm$ 0.69 & 1.0 $\pm$ 0.69 & 1.18 $\pm$ 0.51 & 1.17 $\pm$ 0.58\\
    
    $U_{\it ind}$ & 0.23 $\pm$0.35 & 0.2 $\pm$0.35 & 0.57$\pm$ 0.4 & 0.54$\pm$ 0.41	& 0.56 $\pm$ 0.42 & 0.62 $\pm$ 0.43 & 0.42 $\pm$ 0.25 & 	0.39 $\pm$ 0.26\\
    
    $U_{\it ind}^s$  & \textbf{0.92  $\pm$ 0.2} &\textbf{ 0.92  $\pm$ 0.17 }& 0.81 $\pm$  0.17 & 0.79 $\pm$  0.22 & 0.82 $\pm$ 0.19	 & 0.91 $\pm$ 0.11	 & 0.5 $\pm$ 0.2	 &0.48 $\pm$ 0.19	\\
    
    $P_{\it succ}$ & 0.32 & 0.26 & 0.7 & 0.69 & 0.67 & 0.69 &\textbf{ 0.85} & 0.82\\
    \hline
    \end{tabular}
    }
    \caption{Performance Comparison of \textit{ANESIA} with ``teacher'' strategies. }
    \label{table:teacher1}
\end{table*}


\begin{table*}
    \centering
    \resizebox{.98\textwidth}{!}{
    \begin{tabular}{p{0.14\textwidth} p{0.1\textwidth}p{0.1\textwidth}
    p{0.1\textwidth}p{0.1\textwidth}
    p{0.1\textwidth}p{0.1\textwidth} 
    p{0.1\textwidth}}
    \hline
    \multicolumn{8}{c}{Airport Domain B = 5\% of $\Omega$}\\
    \hline
      Agent &
      $T_{\it avg} (\downarrow)$  &  
      $R_{\it avg} (\downarrow)$  &  
      $P_{\it avg} (\downarrow)$  &  
      $U_{\it soc} (\uparrow)$  &  
      $U_{\it ind}^{total}  (\uparrow)$  &  
      $U_{\it ind}^s  (\uparrow)$  &
       $S_{\%} (\uparrow)$   \\  
      \hline
    ANESIA & 70.6 $\pm$ 66.14 & 938.2 $\pm$ 1487.32 & \textbf{0.01 $\pm$ 0.33} & \textbf{1.65 $\pm$ 0.49} & 0.74 $\pm$ 0.14 &\textbf{ 0.87 $\pm$ 0.11} & 0.89 \\
    AgentGP & 82.67 $\pm$ 72.21 & 825.5 $\pm$ 1754.98 & 0.18 $\pm$ 0.38 & 1.33 $\pm$ 0.57 & 0.78 $\pm$ 0.16 & 0.83 $\pm$ 0.12 & 0.85 \\
    AgentHerb &\textbf{ 0.46 $\pm$ 0.42} & \textbf{8.0 $\pm$ 2.39} & 0.01 $\pm$ 0.05 & 1.58 $\pm$ 0.09 & 0.72 $\pm$ 0.09 & 0.72 $\pm$ 0.09 &\textbf{ 1.0} \\
    FSEGA2019 & 76.56 $\pm$ 57.68 & 3883.13 $\pm$ 8054.86 & 0.1 $\pm$ 0.31 & 1.46 $\pm$ 0.46 & 0.75 $\pm$ 0.13 & 0.78 $\pm$ 0.11 & 0.91 \\
    Agent33 & 62.33 $\pm$ 65.73 & 3037.78 $\pm$ 6336.91 & 0.03 $\pm$ 0.15 & 1.56 $\pm$ 0.23 & 0.73 $\pm$ 0.08 & 0.73 $\pm$ 0.07 & 0.98 \\
    Agent36 & 107.23 $\pm$ 66.23 & 4883.1 $\pm$ 7812.68 & 0.1 $\pm$ 0.31 & 1.44 $\pm$ 0.46 & 0.8 $\pm$ 0.13 & 0.83 $\pm$ 0.1 & 0.91 \\
    Sontag & 45.61 $\pm$ 33.33 & 2476.64 $\pm$ 5562.63 & 0.01 $\pm$ 0.08 & 1.59 $\pm$ 0.13 & 0.77 $\pm$ 0.09 & 0.78 $\pm$ 0.08 & 0.99 \\
    AgreeableAgent & 120.78 $\pm$ 60.53 & 6840.18 $\pm$ 12531.88 & 0.03 $\pm$ 0.15 & 1.55 $\pm$ 0.24 & \textbf{0.85 $\pm$ 0.12} & 0.86 $\pm$ 0.11 & 0.98 \\
    PonpokoAgent & 96.7 $\pm$ 64.33 & 5493.8 $\pm$ 10533.06 & 0.08 $\pm$ 0.28 & 1.47 $\pm$ 0.42 & 0.82 $\pm$ 0.13 & 0.85 $\pm$ 0.09 & 0.93 \\
    ParsCat2 & 73.16 $\pm$ 48.04 & 3483.76 $\pm$ 6177.49 & 0.02 $\pm$ 0.1 & 1.56 $\pm$ 0.16 & 0.78 $\pm$ 0.12 & 0.78 $\pm$ 0.12 & 0.99 \\
        \hline
        \hline
    \multicolumn{8}{c}{Airport Domain B = 10\% of $\Omega$}\\
    \hline
      Agent &
    $T_{\it avg} (\downarrow)$  &  
      $R_{\it avg} (\downarrow)$  &  
      $P_{\it avg} (\downarrow)$  &  
      $U_{\it soc} (\uparrow)$  &  
      $U_{\it ind}^{total}  (\uparrow)$  &  
      $U_{\it ind}^s  (\uparrow)$  &
       $S_{\%} (\uparrow)$   \\    
      \hline
    ANESIA & 71.64 $\pm$ 67.93 & 861.02 $\pm$ 1252.26 & \textbf{0.01 $\pm$ 0.18} & \textbf{1.59 $\pm$ 0.49} & 0.72 $\pm$ 0.2 & \textbf{0.89 $\pm$ 0.1} & 0.87 \\
    AgentGP & 87.37 $\pm$ 64.42 & 606.12 $\pm$ 939.0 & 0.08 $\pm$ 0.15 & 1.04 $\pm$ 0.38 & 0.74 $\pm$ 0.17 & 0.78 $\pm$ 0.11 & 0.93 \\
    AgentHerb & \textbf{0.16 $\pm$ 0.25} & \textbf{3.78 $\pm$ 2.81} & 0.03 $\pm$ 0.07 & 1.5 $\pm$ 0.13 & 0.61 $\pm$ 0.12 & 0.61 $\pm$ 0.12 & 1.00 \\
    FSEGA2019 & 59.95 $\pm$ 40.35 & 2190.82 $\pm$ 3083.94 & 0.01 $\pm$ 0.05 & 1.24 $\pm$ 0.23 & 0.76 $\pm$ 0.14 & 0.77 $\pm$ 0.14 & 0.99 \\
    Agent33 & 12.69 $\pm$ 17.86 & 455.21 $\pm$ 873.55 & 0.03 $\pm$ 0.08 & 1.44 $\pm$ 0.15 & 0.65 $\pm$ 0.13 & 0.65 $\pm$ 0.13 & 1.0 \\
    Agent36 & 97.75 $\pm$ 60.88 & 3191.77 $\pm$ 3918.48 & 0.03 $\pm$ 0.1 & 1.06 $\pm$ 0.31 & 0.81 $\pm$ 0.13 & 0.83 $\pm$ 0.08 & 0.97 \\
    Sontag & 46.63 $\pm$ 36.43 & 1741.54 $\pm$ 2561.66 & 0.01 $\pm$ 0.05 & 1.31 $\pm$ 0.21 & 0.77 $\pm$ 0.12 & 0.77 $\pm$ 0.11 & 0.99 \\
    AgreeableAgent & 106.39 $\pm$ 65.62 & 4196.18 $\pm$ 5275.32 & 0.01 $\pm$ 0.05 & 1.06 $\pm$ 0.32 & \textbf{0.86 $\pm$ 0.13 }& 0.86 $\pm$ 0.12 & 0.99 \\
    PonpokoAgent & 94.14 $\pm$ 65.0 & 3355.75 $\pm$ 4649.12 & 0.04 $\pm$ 0.13 & 1.06 $\pm$ 0.36 & 0.82 $\pm$ 0.16 & 0.85 $\pm$ 0.08 & 0.95 \\
    ParsCat2 & 72.26 $\pm$ 51.6 & 2414.22 $\pm$ 3219.08 & 0.01 $\pm$ 0.05 & 1.19 $\pm$ 0.26 & 0.77 $\pm$ 0.14 & 0.78 $\pm$ 0.13 & 0.99 \\
        \hline
    \end{tabular}
    }
    \caption{AIRPORT (9000 $\times 2$ profiles = 18000 simulations)}
    \label{table:AIRPORT}
\end{table*}



\begin{table*}
    \centering
    \resizebox{.98\textwidth}{!}{
    \begin{tabular}{p{0.14\textwidth} p{0.1\textwidth}p{0.1\textwidth}
    p{0.1\textwidth}p{0.1\textwidth}
    p{0.1\textwidth}p{0.1\textwidth} 
    p{0.1\textwidth}}
    \hline
    \multicolumn{8}{c}{Camera Domain B = 5\% of $\Omega$}\\
    \hline
      Agent &
      $T_{\it avg} (\downarrow)$  &  
      $R_{\it avg} (\downarrow)$  &  
      $P_{\it avg} (\downarrow)$  &  
      $U_{\it soc} (\uparrow)$  &  
      $U_{\it ind}^{total}  (\uparrow)$  &  
      $U_{\it ind}^s  (\uparrow)$  &
       $S_{\%} (\uparrow)$   \\  
      \hline
    ANESIA & 41.36 $\pm$ 25.95 & 3641.0 $\pm$ 716.0 & \textbf{0.02 $\pm$ 0.01} & \textbf{1.38 $\pm$ 0.1} & \textbf{0.88 $\pm$ 0.02} &\textbf{0.88 $\pm$ 0.02} &\textbf{ 1.0 }\\
    AgentGP & 65.73 $\pm$ 71.61 & 70.4 $\pm$ 83.18 & 0.07 $\pm$ 0.06 & 1.36 $\pm$ 0.26 & 0.72 $\pm$ 0.15 & 0.72 $\pm$ 0.15 &\textbf{ 1.0} \\
    AgentHerb & \textbf{0.53 $\pm$ 0.85} & 4\textbf{.81 $\pm$ 1.33 }& 0.03 $\pm$ 0.05 & 1.4 $\pm$ 0.2 & 0.47 $\pm$ 0.19 & 0.47 $\pm$ 0.19 &\textbf{ 1.0} \\
    FSEGA2019 & 86.3 $\pm$ 62.24 & 93.33 $\pm$ 78.91 & 0.14 $\pm$ 0.25 & 1.19 $\pm$ 0.49 & 0.79 $\pm$ 0.14 & 0.83 $\pm$ 0.08 & 0.87 \\
    Agent33 & 41.45 $\pm$ 42.8 & 911.47 $\pm$ 1169.64 & 0.05 $\pm$ 0.06 & 1.37 $\pm$ 0.22 & 0.65 $\pm$ 0.21 & 0.65 $\pm$ 0.21 & \textbf{1.0} \\
    Agent36 & 127.08 $\pm$ 58.78 & 1874.73 $\pm$ 1621.28 & 0.1 $\pm$ 0.18 & 1.12 $\pm$ 0.35 & 0.84 $\pm$ 0.11 & 0.87 $\pm$ 0.06 & 0.93 \\
    Sontag & 60.01 $\pm$ 55.26 & 1198.93 $\pm$ 1352.71 & 0.1 $\pm$ 0.19 & 1.31 $\pm$ 0.39 & 0.71 $\pm$ 0.17 & 0.72 $\pm$ 0.16 & 0.93 \\
    AgreeableAgent & 130.39 $\pm$ 62.8 & 3009.54 $\pm$ 2977.48 & 0.08 $\pm$ 0.2 & 1.15 $\pm$ 0.37 & 0.8 $\pm$ 0.14 & 0.82 $\pm$ 0.12 & 0.92 \\
    PonpokoAgent & 115.17 $\pm$ 60.46 & 2242.19 $\pm$ 2219.61 & 0.1 $\pm$ 0.18 & 1.16 $\pm$ 0.33 & 0.83 $\pm$ 0.14 & 0.85 $\pm$ 0.11 & 0.94 \\
    ParsCat2 & 72.52 $\pm$ 56.32 & 2110.25 $\pm$ 2510.88 & 0.05 $\pm$ 0.06 & 1.36 $\pm$ 0.21 & 0.78 $\pm$ 0.16 & 0.78 $\pm$ 0.16 & \textbf{1.0 }\\



        \hline
        \hline
    \multicolumn{8}{c}{Camera Domain B = 10\% of $\Omega$}\\
    \hline
      Agent &
$T_{\it avg} (\downarrow)$  &  
      $R_{\it avg} (\downarrow)$  &  
      $P_{\it avg} (\downarrow)$  &  
      $U_{\it soc} (\uparrow)$  &  
      $U_{\it ind}^{total}  (\uparrow)$  &  
      $U_{\it ind}^s  (\uparrow)$  &
       $S_{\%} (\uparrow)$   \\  
      \hline

    ANESIA & 100.26 $\pm$ 112.79 & 3541.44 $\pm$ 2993.08 & \textbf{0.02 $\pm$ 0.16 }&\textbf{ 1.86 $\pm$ 0.41} & 0.72 $\pm$ 0.28 &\textbf{ 0.89 $\pm$ 0.09} & 0.88 \\
    AgentGP & 122.19 $\pm$ 108.43 & 297.28 $\pm$ 1032.56 & 0.08 $\pm$ 0.11 & 1.15 $\pm$ 0.33 & 0.73 $\pm$ 0.15 & 0.75 $\pm$ 0.09 & 0.98 \\
    AgentHerb &\textbf{ 0.7 $\pm$ 0.72} & \textbf{3.24 $\pm$ 0.6} & 0.05 $\pm$ 0.08 & 1.44 $\pm$ 0.12 & 0.54 $\pm$ 0.09 & 0.54 $\pm$ 0.09 &\textbf{ 1.0} \\
    FSEGA2019 & 135.97 $\pm$ 87.16 & 289.95 $\pm$ 257.76 & 0.02 $\pm$ 0.06 & 1.18 $\pm$ 0.25 & 0.79 $\pm$ 0.13 & 0.8 $\pm$ 0.11 & 0.99 \\
    Agent33 & 34.59 $\pm$ 29.74 & 2873.5 $\pm$ 3037.28 & 0.05 $\pm$ 0.07 & 1.42 $\pm$ 0.12 & 0.68 $\pm$ 0.12 & 0.68 $\pm$ 0.12 & \textbf{1.0} \\
    Agent36 & 101.72 $\pm$ 101.55 & 8967.21 $\pm$ 7901.54 & 0.03 $\pm$ 0.06 & 1.01 $\pm$ 0.25 & 0.86 $\pm$ 0.11 & 0.87 $\pm$ 0.07 & 0.99 \\
    Sontag & 112.02 $\pm$ 87.37 & 12579.62 $\pm$ 17658.99 & 0.03 $\pm$ 0.06 & 1.24 $\pm$ 0.25 & 0.79 $\pm$ 0.11 & 0.79 $\pm$ 0.11 & \textbf{1.0} \\
    AgreeableAgent & 207.63 $\pm$ 108.52 & 20496.21 $\pm$ 22847.69 & 0.02 $\pm$ 0.04 & 0.98 $\pm$ 0.28 & 0.83 $\pm$ 0.16 & 0.83 $\pm$ 0.16 & \textbf{1.0} \\
    PonpokoAgent & 173.98 $\pm$ 105.66 & 15750.78 $\pm$ 19697.73 & 0.03 $\pm$ 0.06 & 1.06 $\pm$ 0.28 & \textbf{0.88 $\pm$ 0.11} & 0.88 $\pm$ 0.08 & 0.99 \\
    ParsCat2 & 135.34 $\pm$ 91.73 & 9108.99 $\pm$ 11325.86 & 0.04 $\pm$ 0.06 & 1.17 $\pm$ 0.25 & 0.79 $\pm$ 0.11 & 0.79 $\pm$ 0.11 & \textbf{1.0} \\


        \hline
    \end{tabular}
    }
    \caption{CAMERA  (9000 $\times 2$ profiles = 18000 simulations)}
    \label{table:CAMERA}
\end{table*}

\begin{table*}
    \centering
    \resizebox{.98\textwidth}{!}{
    \begin{tabular}{p{0.14\textwidth} p{0.1\textwidth}p{0.1\textwidth}
    p{0.1\textwidth}p{0.1\textwidth}
    p{0.1\textwidth}p{0.1\textwidth} 
    p{0.1\textwidth}}
    \hline
    \multicolumn{8}{c}{Energy Domain B = 5\% of $\Omega$}\\
    \hline
      Agent &
$T_{\it avg} (\downarrow)$  &  
      $R_{\it avg} (\downarrow)$  &  
      $P_{\it avg} (\downarrow)$  &  
      $U_{\it soc} (\uparrow)$  &  
      $U_{\it ind}^{total}  (\uparrow)$  &  
      $U_{\it ind}^s  (\uparrow)$  &
       $S_{\%} (\uparrow)$   \\  
      \hline

    ANESIA & 114.56 $\pm$ 74.17 & 4717.18 $\pm$ 3955.6 & \textbf{0.06 $\pm$ 0.53} &\textbf{ 1.17 $\pm$ 0.75} & 0.61 $\pm$ 0.39 & \textbf{0.85 $\pm$ 0.1} & 0.71 \\
    AgentGP & 129.21 $\pm$ 64.5 & 170.52 $\pm$ 344.74 & 0.34 $\pm$ 0.29 & 0.6 $\pm$ 0.48 & 0.52 $\pm$ 0.12 & 0.54 $\pm$ 0.16 & 0.61 \\
    AgentHerb & \textbf{16.86 $\pm$ 23.04 }& \textbf{75.92 $\pm$ 138.32} & 0.06 $\pm$ 0.08 & 1.05 $\pm$ 0.12 & 0.19 $\pm$ 0.17 & 0.19 $\pm$ 0.17 & \textbf{1.0 }\\
    FSEGA2019 & 148.08 $\pm$ 62.29 & 122.31 $\pm$ 64.47 & 0.53 $\pm$ 0.28 & 0.24 $\pm$ 0.44 & 0.6 $\pm$ 0.19 & 0.93 $\pm$ 0.04 & 0.24 \\
    Agent33 & 115.2 $\pm$ 68.4 & 3626.54 $\pm$ 7173.45 & 0.2 $\pm$ 0.24 & 0.82 $\pm$ 0.41 & 0.5 $\pm$ 0.15 & 0.5 $\pm$ 0.16 & 0.83 \\
    Agent36 & 150.63 $\pm$ 60.24 & 1136.27 $\pm$ 876.21 & 0.47 $\pm$ 0.31 & 0.33 $\pm$ 0.45 & 0.63 $\pm$ 0.19 & 0.87 $\pm$ 0.12 & 0.35 \\
    Sontag & 123.19 $\pm$ 67.93 & 3864.42 $\pm$ 8598.55 & 0.3 $\pm$ 0.3 & 0.62 $\pm$ 0.48 & \textbf{0.67 $\pm$ 0.17 }& 0.76 $\pm$ 0.14 & 0.63 \\
    AgreeableAgent & 155.64 $\pm$ 53.3 & 5304.19 $\pm$ 10699.39 & 0.4 $\pm$ 0.31 & 0.42 $\pm$ 0.44 & 0.62 $\pm$ 0.19 & 0.75 $\pm$ 0.21 & 0.48 \\
    PonpokoAgent & 145.92 $\pm$ 67.78 & 3582.94 $\pm$ 5825.54 & 0.53 $\pm$ 0.28 & 0.25 $\pm$ 0.44 & 0.6 $\pm$ 0.19 & 0.82 $\pm$ 0.1 & 0.25 \\
    Parscat2 & 134.19 $\pm$ 62.76 & 3461.45 $\pm$ 5246.74 & 0.34 $\pm$ 0.3 & 0.57 $\pm$ 0.49 & 0.61 $\pm$ 0.17 & 0.69 $\pm$ 0.19 & 0.58 \\

        \hline
        \hline
    \multicolumn{8}{c}{Energy Domain B = 10\% of $\Omega$}\\
    \hline
      Agent &
$T_{\it avg} (\downarrow)$  &  
      $R_{\it avg} (\downarrow)$  &  
      $P_{\it avg} (\downarrow)$  &  
      $U_{\it soc} (\uparrow)$  &  
      $U_{\it ind}^{total}  (\uparrow)$  &  
      $U_{\it ind}^s  (\uparrow)$  &
       $S_{\%} (\uparrow)$   \\  
      \hline

    ANESIA & 98.93 $\pm$ 69.48 & 4708.91 $\pm$ 3781.56 & \textbf{0.03 $\pm$ 0.41 }& \textbf{1.35 $\pm$ 0.59} &\textbf{ 0.71 $\pm$ 0.31} & \textbf{0.89 $\pm$ 0.11 }& 0.85 \\
    AgentGP & 156.03 $\pm$ 41.87 & 91.36 $\pm$ 237.36 & 0.59 $\pm$ 0.39 & 0.47 $\pm$ 0.56 & 0.41 $\pm$ 0.21 & 0.61 $\pm$ 0.16 & 0.43 \\
    AgentHerb & \textbf{20.2 $\pm$ 29.0} &\textbf{42.41 $\pm$ 28.18 }& 0.07 $\pm$ 0.08 & 1.05 $\pm$ 0.11 & 0.18 $\pm$ 0.16 & 0.18 $\pm$ 0.16 & \textbf{1.0} \\
    FSEGA2019 & 151.22 $\pm$ 58.68 & 124.56 $\pm$ 65.24 & 0.62 $\pm$ 0.4 & 0.38 $\pm$ 0.53 & 0.47 $\pm$ 0.3 & 0.88 $\pm$ 0.07 & 0.35 \\
    Agent33 & 141.49 $\pm$ 56.87 & 3526.95 $\pm$ 4583.61 & 0.19 $\pm$ 0.25 & 1.02 $\pm$ 0.35 & 0.39 $\pm$ 0.17 & 0.4 $\pm$ 0.17 & 0.91 \\
    Agent36 & 148.34 $\pm$ 62.92 & 1111.66 $\pm$ 868.73 & 0.58 $\pm$ 0.42 & 0.42 $\pm$ 0.53 & 0.5 $\pm$ 0.32 & 0.9 $\pm$ 0.08 & 0.39 \\
    Sontag & 139.77 $\pm$ 59.88 & 4042.24 $\pm$ 5517.71 & 0.4 $\pm$ 0.38 & 0.72 $\pm$ 0.52 & 0.57 $\pm$ 0.26 & 0.73 $\pm$ 0.16 & 0.67 \\
    AgreeableAgent & 155.13 $\pm$ 56.98 & 7512.04 $\pm$ 16374.99 & 0.26 $\pm$ 0.32 & 0.87 $\pm$ 0.42 & 0.45 $\pm$ 0.28 & 0.5 $\pm$ 0.3 & 0.82 \\
    PonpokoAgent & 150.86 $\pm$ 62.26 & 7622.98 $\pm$ 17521.91 & 0.47 $\pm$ 0.42 & 0.57 $\pm$ 0.54 & 0.58 $\pm$ 0.32 & 0.88 $\pm$ 0.09 & 0.53 \\
    Parscat2 & 142.17 $\pm$ 60.16 & 3764.06 $\pm$ 4729.56 & 0.39 $\pm$ 0.36 & 0.73 $\pm$ 0.5 & 0.54 $\pm$ 0.24 & 0.66 $\pm$ 0.18 & 0.69 \\

        \hline
    \end{tabular}
    }
    \caption{ENERGY  (9000 $\times 2$ profiles = 18000 simulations)}
    \label{table:ENERGY}
\end{table*}


\begin{table*}
    \centering
    \resizebox{.98\textwidth}{!}{
    \begin{tabular}{p{0.14\textwidth} p{0.1\textwidth}p{0.1\textwidth}
    p{0.1\textwidth}p{0.1\textwidth}
    p{0.1\textwidth}p{0.1\textwidth} 
    p{0.1\textwidth}}
    \hline
    \multicolumn{8}{c}{Fitness Domain = 5\% of $\Omega$}\\
    \hline
      Agent &
$T_{\it avg} (\downarrow)$  &  
      $R_{\it avg} (\downarrow)$  &  
      $P_{\it avg} (\downarrow)$  &  
      $U_{\it soc} (\uparrow)$  &  
      $U_{\it ind}^{total}  (\uparrow)$  &  
      $U_{\it ind}^s  (\uparrow)$  &
       $S_{\%} (\uparrow)$   \\  
      \hline
    ANESIA &\textbf{ 0.78 $\pm$ 0.71} & \textbf{4.76 $\pm$ 2.49} & 0.08 $\pm$ 0.07 & \textbf{1.48 $\pm$ 0.1} & \textbf{0.85 $\pm$ 0.08} & \textbf{0.85 $\pm$ 0.08} & \textbf{1.0} \\
    AgentGP & 85.32 $\pm$ 103.18 & 184.25 $\pm$ 762.86 & \textbf{0.06 $\pm$ 0.04} & 1.37 $\pm$ 0.14 & 0.7 $\pm$ 0.12 & 0.7 $\pm$ 0.12 & \textbf{1.0} \\
    AgentHerb & 0.88 $\pm$ 0.7 & 5.12 $\pm$ 2.08 & \textbf{0.06 $\pm$ 0.1} & 1.47 $\pm$ 0.14 & 0.57 $\pm$ 0.1 & 0.57 $\pm$ 0.1 & 0.99 \\
    FSEGA2019 & 43.31 $\pm$ 37.17 & 3557.81 $\pm$ 4146.44 & 0.08 $\pm$ 0.02 & 1.4 $\pm$ 0.07 & 0.76 $\pm$ 0.13 & 0.76 $\pm$ 0.13 & \textbf{1.0} \\
    Agent33 & 19.79 $\pm$ 15.96 & 1854.04 $\pm$ 2576.79 & 0.08 $\pm$ 0.04 & 1.44 $\pm$ 0.07 & 0.72 $\pm$ 0.13 & 0.72 $\pm$ 0.13 & \textbf{1.0} \\
    Agent36 & 220.89 $\pm$ 90.97 & 11085.16 $\pm$ 8272.13 & 0.07 $\pm$ 0.12 & 1.17 $\pm$ 0.17 & 0.84 $\pm$ 0.15 & 0.84 $\pm$ 0.14 & 0.99 \\
    Sontag & 58.22 $\pm$ 69.85 & 5136.53 $\pm$ 5830.4 & 0.08 $\pm$ 0.03 & 1.38 $\pm$ 0.09 & 0.72 $\pm$ 0.14 & 0.72 $\pm$ 0.14 & \textbf{1.0} \\
    AgreeableAgent & 110.93 $\pm$ 53.37 & 26122.71 $\pm$ 23683.21 & 0.23 $\pm$ 0.1 & 1.51 $\pm$ 0.13 & 0.81 $\pm$ 0.11 & 0.81 $\pm$ 0.11 & \textbf{1.0} \\
    PonpokoAgent & 107.4 $\pm$ 92.69 & 9353.87 $\pm$ 8536.38 & 0.08 $\pm$ 0.02 & 1.31 $\pm$ 0.12 & 0.83 $\pm$ 0.1 & 0.83 $\pm$ 0.1 & \textbf{1.0} \\
    Parscat2 & 91.0 $\pm$ 89.43 & 7456.6 $\pm$ 7936.38 & 0.08 $\pm$ 0.03 & 1.33 $\pm$ 0.1 & 0.74 $\pm$ 0.13 & 0.74 $\pm$ 0.13 & \textbf{1.0} \\

        \hline
        \hline
    \multicolumn{8}{c}{Airport Domain B = 10\% of $\Omega$}\\
    \hline
      Agent &
$T_{\it avg} (\downarrow)$  &  
      $R_{\it avg} (\downarrow)$  &  
      $P_{\it avg} (\downarrow)$  &  
      $U_{\it soc} (\uparrow)$  &  
      $U_{\it ind}^{total}  (\uparrow)$  &  
      $U_{\it ind}^s  (\uparrow)$  &
       $S_{\%} (\uparrow)$   \\  
      \hline
ANESIA & \textbf{1.12 $\pm$ 0.83} & \textbf{7.47 $\pm$ 2.6 }& \textbf{0.04 $\pm$ 0.02} & \textbf{1.62 $\pm$ 0.04} & \textbf{0.86 $\pm$ 0.07} & \textbf{0.86 $\pm$ 0.07} & \textbf{1.0} \\
    AgentGP & 101.04 $\pm$ 114.3 & 147.98 $\pm$ 475.74 & 0.09 $\pm$ 0.04 & 1.46 $\pm$ 0.06 & 0.71 $\pm$ 0.1 & 0.71 $\pm$ 0.1 & \textbf{1.0} \\
    AgentHerb & 1.45 $\pm$ 2.29 & 8.61 $\pm$ 2.46 & 0.09 $\pm$ 0.16 & 1.45 $\pm$ 0.22 & 0.61 $\pm$ 0.1 & 0.61 $\pm$ 0.08 & 0.98 \\
    FSEGA2019 & 49.14 $\pm$ 37.03 & 4213.62 $\pm$ 5498.95 & 0.06 $\pm$ 0.03 & 1.5 $\pm$ 0.04 & 0.76 $\pm$ 0.11 & 0.76 $\pm$ 0.11 & \textbf{1.0} \\
    Agent33 & 112.59 $\pm$ 95.3 & 10684.76 $\pm$ 12674.11 & 0.08 $\pm$ 0.05 & 1.46 $\pm$ 0.07 & 0.82 $\pm$ 0.08 & 0.82 $\pm$ 0.08 & \textbf{1.0} \\
    Agent36 & 234.94 $\pm$ 72.84 & 12468.42 $\pm$ 7653.6 & 0.1 $\pm$ 0.21 & 1.43 $\pm$ 0.29 & 0.78 $\pm$ 0.18 & 0.8 $\pm$ 0.15 & 0.96 \\
    Sontag & 63.71 $\pm$ 71.42 & 6279.91 $\pm$ 7122.37 & 0.07 $\pm$ 0.04 & 1.49 $\pm$ 0.06 & 0.71 $\pm$ 0.12 & 0.71 $\pm$ 0.12 & \textbf{1.0} \\
    AgreeableAgent & 128.81 $\pm$ 58.6 & 24739.93 $\pm$ 26475.48 & 0.15 $\pm$ 0.12 & 1.61 $\pm$ 0.16 & 0.86 $\pm$ 0.12 & 0.86 $\pm$ 0.11 & \textbf{1.0} \\
    PonpokoAgent & 122.93 $\pm$ 98.04 & 11960.5 $\pm$ 12050.08 & 0.06 $\pm$ 0.04 & 1.49 $\pm$ 0.05 & 0.79 $\pm$ 0.1 & 0.79 $\pm$ 0.1 & \textbf{1.0} \\
    Parscat2 & 105.58 $\pm$ 89.28 & 9715.13 $\pm$ 9257.83 & 0.06 $\pm$ 0.04 & 1.49 $\pm$ 0.05 & 0.75 $\pm$ 0.12 & 0.75 $\pm$ 0.12 & \textbf{1.0} \\


        \hline
    \end{tabular}
    }
    \caption{Fitness  (9000 $\times 2$ profiles = 18000 simulations)}
    \label{table:Fitness}
\end{table*}

\begin{table*}
    \centering
    \resizebox{.98\textwidth}{!}{
    \begin{tabular}{p{0.14\textwidth} p{0.1\textwidth}p{0.1\textwidth}
    p{0.1\textwidth}p{0.1\textwidth}
    p{0.1\textwidth}p{0.1\textwidth} 
    p{0.1\textwidth}}
    \hline
    \multicolumn{8}{c}{Flight Domain B = 5\% of $\Omega$}\\
    \hline
      Agent &
    $T_{\it avg} (\downarrow)$  &  
      $R_{\it avg} (\downarrow)$  &  
      $P_{\it avg} (\downarrow)$  &  
      $U_{\it soc} (\uparrow)$  &  
      $U_{\it ind}^{total}  (\uparrow)$  &  
      $U_{\it ind}^s  (\uparrow)$  &
       $S_{\%} (\uparrow)$   \\  
      \hline
ANESIA & 76.71 $\pm$ 77.08 & 1186.7 $\pm$ 2054.2 & \textbf{0.09 $\pm$ 0.24} &\textbf{ 1.29 $\pm$ 0.57} &\textbf{ 0.79 $\pm$ 0.23 }&\textbf{ 0.89 $\pm$ 0.17} & 0.72 \\
    AgentGP & 67.87 $\pm$ 82.27 & 574.32 $\pm$ 751.38 & 0.27 $\pm$ 0.22 & 0.87 $\pm$ 0.61 & 0.74 $\pm$ 0.19 & 0.85 $\pm$ 0.11 & 0.68 \\
    AgentHerb & \textbf{2.44 $\pm$ 13.14} & \textbf{98.43 $\pm$ 553.6} & 0.08 $\pm$ 0.07 & 1.32 $\pm$ 0.08 & 0.58 $\pm$ 0.28 & 0.58 $\pm$ 0.28 & \textbf{1.00 }\\
    FSEGA2019 & 57.31 $\pm$ 68.31 & 3764.38 $\pm$ 8150.0 & 0.11 $\pm$ 0.16 & 1.06 $\pm$ 0.37 & 0.62 $\pm$ 0.29 & 0.63 $\pm$ 0.3 & 0.91 \\
    Agent33 & 13.55 $\pm$ 42.58 & 282.19 $\pm$ 747.34 & 0.09 $\pm$ 0.14 & 1.23 $\pm$ 0.31 & 0.59 $\pm$ 0.29 & 0.6 $\pm$ 0.3 & 0.94 \\
    Agent36 & 20.9 $\pm$ 53.42 & 323.62 $\pm$ 865.54 & 0.12 $\pm$ 0.15 & 1.19 $\pm$ 0.35 & 0.64 $\pm$ 0.28 & 0.65 $\pm$ 0.29 & 0.93 \\
    Sontag & 42.99 $\pm$ 50.28 & 3244.7 $\pm$ 5039.65 & 0.11 $\pm$ 0.14 & 1.14 $\pm$ 0.3 & 0.61 $\pm$ 0.28 & 0.61 $\pm$ 0.29 & 0.94 \\
    AgreeableAgent & 53.33 $\pm$ 68.46 & 4482.69 $\pm$ 8625.51 & 0.13 $\pm$ 0.17 & 1.06 $\pm$ 0.4 & 0.62 $\pm$ 0.29 & 0.64 $\pm$ 0.3 & 0.89 \\
    PonpokoAgent & 40.6 $\pm$ 62.94 & 1776.02 $\pm$ 3728.31 & 0.12 $\pm$ 0.16 & 1.15 $\pm$ 0.4 & 0.68 $\pm$ 0.24 & 0.7 $\pm$ 0.24 & 0.9 \\
    ParsCat2 & 27.64 $\pm$ 46.3 & 2055.99 $\pm$ 4759.74 & 0.09 $\pm$ 0.09 & 1.22 $\pm$ 0.2 & 0.6 $\pm$ 0.27 & 0.6 $\pm$ 0.28 & 0.99 \\
        \hline
        \hline
    \multicolumn{8}{c}{Flight Domain B = 10\% of $\Omega$}\\
    \hline
      Agent &
$T_{\it avg} (\downarrow)$  &  
      $R_{\it avg} (\downarrow)$  &  
      $P_{\it avg} (\downarrow)$  &  
      $U_{\it soc} (\uparrow)$  &  
      $U_{\it ind}^{total}  (\uparrow)$  &  
      $U_{\it ind}^s  (\uparrow)$  &
       $S_{\%} (\uparrow)$   \\  
      \hline

    ANESIA & 59.14 $\pm$ 66.8 & 520.64 $\pm$ 686.99 & \textbf{0.14 $\pm$ 0.23} & \textbf{1.32 $\pm$ 0.39} &\textbf{ 0.86 $\pm$ 0.22} & \textbf{0.93 $\pm$ 0.1} & 0.9 \\
    AgentGP & 42.98 $\pm$ 72.54 & 243.33 $\pm$ 429.1 & 0.18 $\pm$ 0.21 & 1.14 $\pm$ 0.37 & 0.84 $\pm$ 0.2 & 0.9 $\pm$ 0.05 & 0.91 \\
    AgentHerb & \textbf{0.24 $\pm$ 0.25} & \textbf{4.47 $\pm$ 2.08} & 0.14 $\pm$ 0.07 & 1.26 $\pm$ 0.11 & 0.74 $\pm$ 0.23 & 0.74 $\pm$ 0.23 &\textbf{ 1.00} \\
    FSEGA2019 & 40.0 $\pm$ 46.12 & 1069.13 $\pm$ 1692.4 & 0.18 $\pm$ 0.1 & 1.18 $\pm$ 0.15 & 0.48 $\pm$ 0.19 & 0.48 $\pm$ 0.19 & \textbf{1.00} \\
    Agent33 & 47.55 $\pm$ 63.91 & 1214.26 $\pm$ 2160.5 & 0.17 $\pm$ 0.13 & 1.19 $\pm$ 0.2 & 0.63 $\pm$ 0.22 & 0.64 $\pm$ 0.22 & 0.99 \\
    Agent36 & 83.08 $\pm$ 64.9 & 1921.63 $\pm$ 2271.83 & 0.2 $\pm$ 0.13 & 1.12 $\pm$ 0.21 & 0.45 $\pm$ 0.15 & 0.46 $\pm$ 0.15 & 0.98 \\
    Sontag & 20.25 $\pm$ 18.84 & 530.21 $\pm$ 607.27 & 0.17 $\pm$ 0.09 & 1.2 $\pm$ 0.13 & 0.59 $\pm$ 0.23 & 0.59 $\pm$ 0.23 & \textbf{1.00} \\
    AgreeableAgent & 70.35 $\pm$ 67.21 & 2003.06 $\pm$ 2668.01 & 0.15 $\pm$ 0.07 & 1.19 $\pm$ 0.13 & 0.45 $\pm$ 0.17 & 0.45 $\pm$ 0.17 &\textbf{ 1.00} \\
    PonpokoAgent & 61.96 $\pm$ 61.78 & 1713.98 $\pm$ 2426.42 & 0.2 $\pm$ 0.14 & 1.13 $\pm$ 0.24 & 0.49 $\pm$ 0.17 & 0.49 $\pm$ 0.17 & 0.97 \\
    ParsCat2 & 18.62 $\pm$ 24.79 & 404.32 $\pm$ 435.13 & 0.17 $\pm$ 0.08 & 1.2 $\pm$ 0.12 & 0.59 $\pm$ 0.24 & 0.59 $\pm$ 0.24 & \textbf{1.00} \\
        \hline
    \end{tabular}
    }
    \caption{Flight  (9000 $\times 2$ profiles = 18000 simulations)}
    \label{table:Flight}
\end{table*}

\begin{table*}
    \centering
    \resizebox{.98\textwidth}{!}{
    \begin{tabular}{p{0.14\textwidth} p{0.1\textwidth}p{0.1\textwidth}
    p{0.1\textwidth}p{0.1\textwidth}
    p{0.1\textwidth}p{0.1\textwidth} 
    p{0.1\textwidth}}
    \hline
    \multicolumn{8}{c}{Grocery Domain B = 5\% of $\Omega$}\\
    \hline
      Agent &
$T_{\it avg} (\downarrow)$  &  
      $R_{\it avg} (\downarrow)$  &  
      $P_{\it avg} (\downarrow)$  &  
      $U_{\it soc} (\uparrow)$  &  
      $U_{\it ind}^{total}  (\uparrow)$  &  
      $U_{\it ind}^s  (\uparrow)$  &
       $S_{\%} (\uparrow)$   \\  
      \hline
    ANESIA & 100.23 $\pm$ 75.06 & 679.62 $\pm$ 657.18 & \textbf{0.03 $\pm$ 0.35} & \textbf{1.29 $\pm$ 0.65} & 0.5 $\pm$ 0.39 & \textbf{0.86 $\pm$ 0.25} & 0.69 \\
    AgentGP & 89.16 $\pm$ 66.41 & 189.07 $\pm$ 146.98 & 0.21 $\pm$ 0.2 & 1.14 $\pm$ 0.39 & 0.6 $\pm$ 0.21 & 0.64 $\pm$ 0.14 & 0.93 \\
    AgentHerb & \textbf{0.48 $\pm$ 0.43} & \textbf{6.12 $\pm$ 2.35} & 0.12 $\pm$ 0.09 & 1.37 $\pm$ 0.13 & 0.49 $\pm$ 0.11 & 0.49 $\pm$ 0.11 & \textbf{1.00} \\
    FSEGA2019 & 79.5 $\pm$ 59.65 & 1232.33 $\pm$ 1446.09 & 0.19 $\pm$ 0.19 & 1.16 $\pm$ 0.34 & 0.7 $\pm$ 0.21 & 0.74 $\pm$ 0.13 & 0.94 \\
    Agent33 & 41.3 $\pm$ 49.27 & 603.12 $\pm$ 708.77 & 0.14 $\pm$ 0.19 & 1.31 $\pm$ 0.35 & 0.57 $\pm$ 0.18 & 0.61 $\pm$ 0.12 & 0.94 \\
    Agent36 & 125.47 $\pm$ 59.54 & 3063.11 $\pm$ 2748.19 & 0.19 $\pm$ 0.23 & 1.07 $\pm$ 0.4 & \textbf{0.75 $\pm$ 0.28} & 0.84 $\pm$ 0.1 & 0.89 \\
    Sontag & 83.09 $\pm$ 65.85 & 2116.71 $\pm$ 2459.88 & 0.25 $\pm$ 0.27 & 1.09 $\pm$ 0.52 & 0.61 $\pm$ 0.31 & 0.74 $\pm$ 0.13 & 0.82 \\
    AgreeableAgent & 137.36 $\pm$ 62.14 & 2961.29 $\pm$ 2861.58 & 0.23 $\pm$ 0.23 & 0.98 $\pm$ 0.4 & 0.65 $\pm$ 0.28 & 0.74 $\pm$ 0.16 & 0.88 \\
    PonpokoAgent & 106.64 $\pm$ 65.09 & 3430.65 $\pm$ 3077.45 & 0.19 $\pm$ 0.24 & 1.09 $\pm$ 0.42 & 0.76 $\pm$ 0.29 & \textbf{0.86 $\pm$ 0.09} & 0.88 \\
    Parscat2 & 99.85 $\pm$ 61.05 & 1935.62 $\pm$ 1612.92 & 0.1 $\pm$ 0.07 & 1.28 $\pm$ 0.12 & 0.77 $\pm$ 0.12 & 0.77 $\pm$ 0.12 & \textbf{1.00} \\

        \hline
        \hline
    \multicolumn{8}{c}{Grocery Domain B = 10\% of $\Omega$}\\
    \hline
      Agent &
$T_{\it avg} (\downarrow)$  &  
      $R_{\it avg} (\downarrow)$  &  
      $P_{\it avg} (\downarrow)$  &  
      $U_{\it soc} (\uparrow)$  &  
      $U_{\it ind}^{total}  (\uparrow)$  &  
      $U_{\it ind}^s  (\uparrow)$  &
       $S_{\%} (\uparrow)$   \\  
      \hline
    ANESIA & 123.62 $\pm$ 67.47 & 1891.11 $\pm$ 2003.69 &\textbf{ 0.06 $\pm$ 0.08} & \textbf{1.63 $\pm$ 0.74} &  \textbf{0.86 $\pm$ 0.12} & \textbf{0.86 $\pm$ 0.12} & 0.67 \\
    AgentGP & 79.86 $\pm$ 64.52 & 282.6 $\pm$ 531.88 & 0.19 $\pm$ 0.23 & 1.37 $\pm$ 0.36 & 0.64 $\pm$ 0.15 & 0.64 $\pm$ 0.15 & 0.95 \\
    AgentHerb & \textbf{0.75 $\pm$ 0.77} & \textbf{9.55 $\pm$ 2.4} & 0.11 $\pm$ 0.07 & 1.41 $\pm$ 0.14 & 0.51 $\pm$ 0.15 & 0.51 $\pm$ 0.15 & \textbf{1.00} \\
    FSEGA2019 & 79.94 $\pm$ 45.22 & 1970.04 $\pm$ 2522.56 & 0.12 $\pm$ 0.12 & 1.49 $\pm$ 0.2 & 0.74 $\pm$ 0.1 & 0.74 $\pm$ 0.1 & 0.99 \\
    Agent33 & 106.31 $\pm$ 59.73 & 4151.6 $\pm$ 5465.27 & 0.08 $\pm$ 0.17 & 1.56 $\pm$ 0.27 & 0.82 $\pm$ 0.14 & 0.83 $\pm$ 0.13 & 0.98 \\
    Agent36 & 132.29 $\pm$ 55.72 & 3868.66 $\pm$ 3914.42 & 0.13 $\pm$ 0.21 & 1.47 $\pm$ 0.33 & 0.84 $\pm$ 0.13 & 0.85 $\pm$ 0.12 & 0.96 \\
    Sontag & 75.0 $\pm$ 46.85 & 3124.65 $\pm$ 4579.55 & 0.1 $\pm$ 0.1 & 1.52 $\pm$ 0.18 & 0.73 $\pm$ 0.12 & 0.73 $\pm$ 0.12 & \textbf{1.00} \\
    AgreeableAgent & 138.03 $\pm$ 52.91 & 5203.96 $\pm$ 6876.31 & 0.17 $\pm$ 0.2 & 1.41 $\pm$ 0.31 & 0.8 $\pm$ 0.13 & 0.81 $\pm$ 0.12 & 0.97 \\
    PonpokoAgent & 116.86 $\pm$ 59.78 & 4613.12 $\pm$ 6604.24 & 0.17 $\pm$ 0.22 & 1.41 $\pm$ 0.33 & 0.82 $\pm$ 0.11 & 0.84 $\pm$ 0.09 & 0.96 \\
    Parscat2 & 98.56 $\pm$ 48.59 & 3412.35 $\pm$ 4350.35 & 0.13 $\pm$ 0.12 & 1.47 $\pm$ 0.18 & 0.74 $\pm$ 0.13 & 0.74 $\pm$ 0.13 & \textbf{1.00} \\

        \hline
    \end{tabular}
    }
    \caption{Grocery  (9000 $\times 2$ profiles = 18000 simulations)}
    \label{table:Grocery}
\end{table*}

\begin{table*}
    \centering
    \resizebox{.98\textwidth}{!}{
    \begin{tabular}{p{0.14\textwidth} p{0.1\textwidth}p{0.1\textwidth}
    p{0.1\textwidth}p{0.1\textwidth}
    p{0.1\textwidth}p{0.1\textwidth} 
    p{0.1\textwidth}}
    \hline
    \multicolumn{8}{c}{Itex Domain B = 5\% of $\Omega$}\\
    \hline
      Agent &
$T_{\it avg} (\downarrow)$  &  
      $R_{\it avg} (\downarrow)$  &  
      $P_{\it avg} (\downarrow)$  &  
      $U_{\it soc} (\uparrow)$  &  
      $U_{\it ind}^{total}  (\uparrow)$  &  
      $U_{\it ind}^s  (\uparrow)$  &
       $S_{\%} (\uparrow)$   \\  
      \hline
    ANESIA & 16.5 $\pm$ 23.52 & 333.5 $\pm$ 660.59 & \textbf{0.03 $\pm$ 0.05} &\textbf{ 1.15 $\pm$ 0.13} &\textbf{ 0.86 $\pm$ 0.29}&\textbf{ 0.86 $\pm$ 0.29} & \textbf{1.0} \\
    AgentGP & 121.16 $\pm$ 78.76 & 758.75 $\pm$ 575.67 & 0.21 $\pm$ 0.2 & 0.54 $\pm$ 0.48 & 0.62 $\pm$ 0.16 & 0.7 $\pm$ 0.17 & 0.6 \\
    AgentHerb &\textbf{2.26 $\pm$ 11.67} & \textbf{9.61 $\pm$ 7.9} & 0.04 $\pm$ 0.07 & 1.14 $\pm$ 0.1 & 0.3 $\pm$ 0.11 & 0.3 $\pm$ 0.11 & \textbf{1.0 }\\
    FSEGA2019 & 105.34 $\pm$ 65.94 & 6853.61 $\pm$ 9301.4 & 0.14 $\pm$ 0.17 & 0.66 $\pm$ 0.39 & 0.68 $\pm$ 0.2 & 0.72 $\pm$ 0.2 & 0.78 \\
    Agent33 & 72.21 $\pm$ 67.93 & 4435.39 $\pm$ 7160.59 & 0.08 $\pm$ 0.12 & 0.88 $\pm$ 0.33 & 0.45 $\pm$ 0.21 & 0.45 $\pm$ 0.22 & 0.93 \\
    Agent36 & 135.67 $\pm$ 67.8 & 6654.0 $\pm$ 7846.72 & 0.13 $\pm$ 0.2 & 0.58 $\pm$ 0.42 & \textbf{0.75 $\pm$ 0.19} & 0.86 $\pm$ 0.11 & 0.71 \\
    Sontag & 112.75 $\pm$ 72.78 & 10871.38 $\pm$ 16140.04 & 0.12 $\pm$ 0.15 & 0.69 $\pm$ 0.38 & 0.57 $\pm$ 0.19 & 0.58 $\pm$ 0.21 & 0.85 \\
    AgreeableAgent & 135.89 $\pm$ 72.22 & 12285.09 $\pm$ 17120.59 & 0.19 $\pm$ 0.2 & 0.51 $\pm$ 0.44 & 0.65 $\pm$ 0.19 & 0.73 $\pm$ 0.2 & 0.64 \\
    PonpokoAgent & 131.54 $\pm$ 72.49 & 7367.07 $\pm$ 10527.99 & 0.23 $\pm$ 0.21 & 0.46 $\pm$ 0.48 & 0.67 $\pm$ 0.19 & 0.85 $\pm$ 0.09 & 0.5 \\
    ParsCat2 & 109.74 $\pm$ 69.98 & 13075.38 $\pm$ 12919.99 & 0.13 $\pm$ 0.18 & 0.65 $\pm$ 0.43 & 0.69 $\pm$ 0.21 & 0.76 $\pm$ 0.2 & 0.75 \\
        \hline
        \hline
    \multicolumn{8}{c}{Itex Domain B = 10\% of $\Omega$}\\
    \hline
      Agent &
    $T_{\it avg} (\downarrow)$  &  
      $R_{\it avg} (\downarrow)$  &  
      $P_{\it avg} (\downarrow)$  &  
      $U_{\it soc} (\uparrow)$  &  
      $U_{\it ind}^{total}  (\uparrow)$  &  
      $U_{\it ind}^s  (\uparrow)$  &
       $S_{\%} (\uparrow)$   \\  
      \hline
    ANESIA & 21.78 $\pm$ 23.77 & 480.76 $\pm$ 887.11 & \textbf{0.03 $\pm$ 0.05} & \textbf{1.13 $\pm$ 0.08} & \textbf{0.83 $\pm$ 0.2} & \textbf{0.83 $\pm$ 0.2} & \textbf{1.0} \\
    AgentGP & 89.03 $\pm$ 71.15 & 702.79 $\pm$ 991.59 & 0.15 $\pm$ 0.21 & 0.85 $\pm$ 0.36 & 0.68 $\pm$ 0.24 & 0.75 $\pm$ 0.18 & 0.86 \\
    AgentHerb & \textbf{0.4 $\pm$ 1.73} &\textbf{ 6.5 $\pm$ 13.38} & 0.11 $\pm$ 0.11 & 1.1 $\pm$ 0.08 & 0.34 $\pm$ 0.15 & 0.34 $\pm$ 0.15 &\textbf{ 1.0} \\
    FSEGA2019 & 60.84 $\pm$ 41.3 & 2501.63 $\pm$ 3598.22 & 0.14 $\pm$ 0.11 & 0.96 $\pm$ 0.11 & 0.54 $\pm$ 0.23 & 0.54 $\pm$ 0.23 & 0.99 \\
    Agent33 & 21.0 $\pm$ 24.88 & 699.03 $\pm$ 1673.14 & 0.15 $\pm$ 0.1 & 1.02 $\pm$ 0.09 & 0.43 $\pm$ 0.19 & 0.43 $\pm$ 0.19 &\textbf{ 1.0} \\
    Agent36 & 86.71 $\pm$ 59.38 & 3459.43 $\pm$ 4660.2 & 0.16 $\pm$ 0.14 & 0.9 $\pm$ 0.22 & 0.51 $\pm$ 0.19 & 0.52 $\pm$ 0.18 & 0.96 \\
    Sontag & 52.35 $\pm$ 43.41 & 2426.79 $\pm$ 4049.43 & 0.14 $\pm$ 0.11 & 0.98 $\pm$ 0.11 & 0.55 $\pm$ 0.24 & 0.55 $\pm$ 0.24 & \textbf{1.0} \\
    AgreeableAgent & 107.63 $\pm$ 62.93 & 4869.51 $\pm$ 6498.22 & 0.14 $\pm$ 0.1 & 0.89 $\pm$ 0.16 & 0.65 $\pm$ 0.23 & 0.66 $\pm$ 0.23 & 0.99 \\
    PonpokoAgent & 88.57 $\pm$ 61.99 & 4094.31 $\pm$ 5775.35 & 0.19 $\pm$ 0.12 & 0.88 $\pm$ 0.19 & 0.52 $\pm$ 0.14 & 0.53 $\pm$ 0.13 & 0.97 \\
    ParsCat2 & 74.45 $\pm$ 53.58 & 2879.83 $\pm$ 4078.87 & 0.16 $\pm$ 0.11 & 0.93 $\pm$ 0.15 & 0.51 $\pm$ 0.18 & 0.52 $\pm$ 0.18 & 0.99 \\
        \hline
    \end{tabular}
    }
    \caption{Itex  (9000 $\times 2$ profiles = 18000 simulations)}
    \label{table:Itex}
\end{table*}


\begin{table*}
    \centering
    \resizebox{.98\textwidth}{!}{
    \begin{tabular}{p{0.14\textwidth} p{0.1\textwidth}p{0.1\textwidth}
    p{0.1\textwidth}p{0.1\textwidth}
    p{0.1\textwidth}p{0.1\textwidth} 
    p{0.1\textwidth}}
    \hline
    \multicolumn{8}{c}{Outfit Domain B = 5\% of $\Omega$}\\
    \hline
      Agent &
$T_{\it avg} (\downarrow)$  &  
      $R_{\it avg} (\downarrow)$  &  
      $P_{\it avg} (\downarrow)$  &  
      $U_{\it soc} (\uparrow)$  &  
      $U_{\it ind}^{total}  (\uparrow)$  &  
      $U_{\it ind}^s  (\uparrow)$  &
       $S_{\%} (\uparrow)$   \\  
      \hline
    ANESIA & 39.17 $\pm$ 45.38 & 372.13 $\pm$ 455.54 &\textbf{ 0.03 $\pm$ 0.13} & \textbf{1.62 $\pm$ 0.4} & \textbf{0.85 $\pm$ 0.16} & \textbf{0.91 $\pm$ 0.13} & 0.93 \\
    AgentGP & 61.03 $\pm$ 62.33 & 482.0 $\pm$ 402.34 & 0.11 $\pm$ 0.17 & 1.19 $\pm$ 0.51 & \textbf{0.85 $\pm$ 0.14} & 0.9 $\pm$ 0.05 & 0.87 \\
    AgentHerb & \textbf{0.11 $\pm$ 0.1} & \textbf{2.94 $\pm$ 0.91} & 0.06 $\pm$ 0.08 & 1.56 $\pm$ 0.13 & 0.62 $\pm$ 0.13 & 0.62 $\pm$ 0.13 & \textbf{1.0} \\
    FESGA2019 & 66.87 $\pm$ 43.77 & 2844.21 $\pm$ 3288.81 & 0.03 $\pm$ 0.04 & 1.23 $\pm$ 0.22 & 0.76 $\pm$ 0.15 & 0.76 $\pm$ 0.15 & \textbf{1.0} \\
    Agent33 & 16.58 $\pm$ 8.89 & 755.56 $\pm$ 576.24 & 0.04 $\pm$ 0.05 & 1.47 $\pm$ 0.14 & 0.65 $\pm$ 0.13 & 0.65 $\pm$ 0.13 & \textbf{1.0} \\
    Agent36 & 97.62 $\pm$ 64.65 & 2925.27 $\pm$ 2243.27 & 0.11 $\pm$ 0.17 & 1.01 $\pm$ 0.46 & 0.78 $\pm$ 0.13 & 0.83 $\pm$ 0.07 & 0.87 \\
    Sontag & 48.67 $\pm$ 42.32 & 1446.14 $\pm$ 1670.97 & 0.05 $\pm$ 0.04 & 1.31 $\pm$ 0.24 & 0.79 $\pm$ 0.14 & 0.79 $\pm$ 0.14 & \textbf{1.0} \\
    AgreeableAgent & 114.62 $\pm$ 69.19 & 3608.79 $\pm$ 3368.0 & 0.05 $\pm$ 0.04 & 1.05 $\pm$ 0.32 & 0.84 $\pm$ 0.11 & 0.84 $\pm$ 0.11 & \textbf{1.0} \\
    PonpokoAgent & 92.59 $\pm$ 64.39 & 3974.12 $\pm$ 3667.82 & 0.08 $\pm$ 0.14 & 1.07 $\pm$ 0.39 & 0.84 $\pm$ 0.14 & 0.86 $\pm$ 0.11 & 0.94 \\
    ParsCat2 & 71.69 $\pm$ 52.92 & 2122.83 $\pm$ 2013.23 & 0.05 $\pm$ 0.04 & 1.22 $\pm$ 0.25 & 0.81 $\pm$ 0.1 & 0.81 $\pm$ 0.1 & \textbf{1.0} \\
        \hline
        \hline
    \multicolumn{8}{c}{Outfit Domain B = 10\% of $\Omega$}\\
    \hline
      Agent &
$T_{\it avg} (\downarrow)$  &  
      $R_{\it avg} (\downarrow)$  &  
      $P_{\it avg} (\downarrow)$  &  
      $U_{\it soc} (\uparrow)$  &  
      $U_{\it ind}^{total}  (\uparrow)$  &  
      $U_{\it ind}^s  (\uparrow)$  &
       $S_{\%} (\uparrow)$   \\  
      \hline
    ANESIA & 16.58 $\pm$ 20.51 & 299.8 $\pm$ 623.92 &\textbf{ 0.09 $\pm$ 0.13} & \textbf{1.43 $\pm$ 0.19} & \textbf{0.88 $\pm$ 0.17} & \textbf{0.88 $\pm$ 0.17} & \textbf{1.0} \\
    AgentGP & 93.04 $\pm$ 68.23 & 761.22 $\pm$ 846.16 & 0.18 $\pm$ 0.26 & 1.17 $\pm$ 0.5 & 0.76 $\pm$ 0.26 & 0.84 $\pm$ 0.17 & 0.87 \\
    AgentHerb & \textbf{0.45 $\pm$ 0.47} & \textbf{8.73 $\pm$ 4.01} & 0.22 $\pm$ 0.1 & 1.35 $\pm$ 0.18 & 0.53 $\pm$ 0.11 & 0.53 $\pm$ 0.11 & \textbf{1.0} \\
    FSEGA2019 & 88.39 $\pm$ 51.19 & 3600.0 $\pm$ 4471.93 & 0.09 $\pm$ 0.11 & 1.32 $\pm$ 0.2 & 0.75 $\pm$ 0.12 & 0.76 $\pm$ 0.11 & 0.99 \\
    Agent33 & 46.14 $\pm$ 46.05 & 2004.92 $\pm$ 3323.93 & 0.14 $\pm$ 0.11 & 1.34 $\pm$ 0.23 & 0.61 $\pm$ 0.15 & 0.61 $\pm$ 0.15 & \textbf{1.0} \\
    Agent36 & 132.62 $\pm$ 61.43 & 5697.88 $\pm$ 6025.18 & 0.2 $\pm$ 0.18 & 1.07 $\pm$ 0.29 & 0.74 $\pm$ 0.16 & 0.77 $\pm$ 0.11 & 0.95 \\
    Sontag & 82.65 $\pm$ 53.76 & 3869.24 $\pm$ 5136.25 & 0.08 $\pm$ 0.09 & 1.35 $\pm$ 0.14 & 0.75 $\pm$ 0.1 & 0.75 $\pm$ 0.1 & \textbf{1.0} \\
    AgreeableAgent & 131.81 $\pm$ 61.09 & 6016.2 $\pm$ 6877.89 & 0.15 $\pm$ 0.15 & 1.14 $\pm$ 0.23 & 0.78 $\pm$ 0.18 & 0.79 $\pm$ 0.17 & 0.98 \\
    PonpokoAgent & 111.05 $\pm$ 63.27 & 4861.47 $\pm$ 5732.4 & 0.15 $\pm$ 0.2 & 1.19 $\pm$ 0.36 & 0.82 $\pm$ 0.18 & 0.87 $\pm$ 0.09 & 0.93 \\
    ParsCat2 & 96.88 $\pm$ 57.8 & 3727.35 $\pm$ 4614.32 & 0.09 $\pm$ 0.1 & 1.31 $\pm$ 0.17 & 0.77 $\pm$ 0.12 & 0.77 $\pm$ 0.11 & \textbf{1.0} \\
        \hline
    \end{tabular}
    }
    \caption{Outfit  (9000 $\times 2$ profiles = 18000 simulations)}
    \label{table:outfit}
\end{table*}
